# Supplementary material for: Sparse-VQ Transformer: An FFN-Free Framework with Vector Quantization for Enhanced Time Series Forecasting
Source: arXiv:2402.05830 source file (2024-02-08)
Supplement: Supplementary file 1 [file 0_appendix_main.tex]

\section{Visualization}

\begin{figure*}[t]
\centering
% \scalebox{0.70}{
\includegraphics[width=0.95\linewidth]{graphs/5_compare_global_local_1.pdf}
\caption{Visualization of 96 step forecasting }
\label{fig:boost}
% \vskip -0.2in
\end{figure*}

\begin{figure*}[t]
\centering
% \scalebox{0.70}{
\includegraphics[width=0.95\linewidth]{graphs/5_compare_global_local_2.pdf}
\caption{.}
\label{fig:boost}
% \vskip -0.2in
\end{figure*}

We visualize the forecasting results of,

We observe that xxx.
