# Supplementary material for: Sparse-VQ Transformer: An FFN-Free Framework with Vector Quantization for Enhanced Time Series Forecasting
Source: arXiv:2402.05830 source file (2024-02-08)
Supplement: Supplementary file 4 [file additional_benchmarks.tex]

\section{Additional Benchmarks}
\subsection{Multivariate long-term series forecasting with extra baseline models}
For the additional benchmarks for multivariate experiments, we add some non-Transformer methods for comparison.N-BEATS\cite{nbeats} and N-HiTS\cite{challu2022n} are two recent proposed powerful non-Transformer methods. As N-HiTS is the latest development from the research group, which also published N-BEATS, we add N-HiTS to our empirical comparison. Here, we adopt the results in the N-HiTS paper to prevent inappropriate parameter tuning problems. We also add a seasonal-naive model in the comparison. FiLM outperforms N-HiTS in most cases(33/48). Moreover, Simple Seasonal-naive\cite{seasonal-naive} is a solid baseline on exchange datasets better than N-hits, Fedformer, and Autoformer, but FiLM still surpasses its performance, as shown in Table \ref{tab:multi-benchmarks}.
%\resizebox{!}{\.5\paperheight}{
% \vskip -0.2in
\begin{table*}[h!]
\centering
%\begin{footnotesize}
% \begin{adjustwidth}{-1.5in}{-1in}
\caption{multivariate long-term series forecasting results on six datasets with various input length and prediction length $O \in \{96,192,336,720\}$ (For ILI dataset, we set prediction length $O \in \{24,36,48,60\}$). Supplementary results of non-Transformer baselines (N-Hits and a seasonal-naive model).}
% \vspace{-1mm}
\scalebox{0.8}{
\begin{tabular}{c|c|cccccccccccccccc|}
\toprule
\multicolumn{2}{c|}{Methods}&\multicolumn{2}{c|}{FiLM}&\multicolumn{2}{c|}{N-Hits}&\multicolumn{2}{c|}{FEDformer}&\multicolumn{2}{c|}{Autoformer}&\multicolumn{2}{c|}{Seasonal-naive}\\
\midrule
\multicolumn{2}{c|}{Metric} & MSE  & MAE & MSE & MAE& MSE  & MAE& MSE  & MAE& MSE  & MAE \\
\midrule
\multirow{4}{*}{\rotatebox{90}{$ETTm2$}} 
                        &96 & \textbf{0.165} & 0.256 & 0.176 & \textbf{0.255} &0.203 &0.287 &0.255  &0.339  &0.262 &0.300 \\
                        & 192 & \textbf{0.222} & \textbf{0.296} & 0.245 & 0.305 & 0.269  &0.328  &0.281 &0.340  &0.319 &0.337\\
                        & 336 & \textbf{0.277} & \textbf{0.333} & 0.295 & 0.346 & 0.325 &0.366 &0.339  &0.372  &0.375 &0.371\\
                        & 720 & \textbf{0.371} & \textbf{0.389} & 0.401 & 0.426 & 0.421 &0.415 &0.422  &0.419 &0.469 &0.422\\
\midrule
\multirow{4}{*}{\rotatebox{90}{$Electricity$}} 
                        &96  &0.154  &0.267 & \textbf{0.147} & \textbf{0.249}  &0.183 &0.297 &0.201  &0.317 &0.211 &0.278\\
                        & 192 &\textbf{0.164} & \textbf{0.258} & 0.167 & 0.269 & 0.195 &0.308 &0.222  &0.334 &0.214 &0.282\\
                        & 336 & 0.188 & \textbf{0.283} & \textbf{0.186} & 0.290 & 0.212 &0.313 &0.231 &0.338 &0.226 &0.294\\
                        & 720 & 0.236 & \textbf{0.332} & 0.243 & 0.340 &\textbf{0.231} &0.343 &0.254  &0.361 &0.265 & 0.324\\
\midrule
\multirow{4}{*}{\rotatebox{90}{$Exchange$}} 
                        &96  & \textbf{0.086} & \textbf{0.204} &0.092 & 0.211 & 0.139 & 0.276 & 0.197 &0.323 &0.086 &0.204 \\
                        & 192 & \textbf{0.189} & \textbf{0.292} & 0.208 & 0.322 &0.256 &0.369 & 0.300 & 0.369 &0.172 &0.295\\
                        & 336 & \textbf{0.356} & \textbf{0.433} & 0.371 & 0.443 & 0.426 &0.464 & 0.509 & 0.524 &0.311 &0.401\\
                        & 720 & \textbf{0.727} & \textbf{0.669} & 0.888 & 0.723 &  1.090 &0.800 & 1.447 & 0.941 &0.832 &0.686\\
\midrule
\multirow{4}{*}{\rotatebox{90}{$Traffic$}} 
                        &96  & 0.416& 0.294 & \textbf{0.402} & \textbf{0.282} & 0.562 &0.349 &0.613  &0.388 &1.219 &0.497\\
                        & 192 & \textbf{0.408} & \textbf{0.288} &0.420 & 0.297 & 0.562 &0.346 &0.616&0.382 &1.089 &0.456\\
                        & 336 & \textbf{0.425} & \textbf{0.298} &0.448 & 0.313 & 0.570 &0.323 &0.622  &0.337 &1.147 &0.473\\
                        & 720 & \textbf{0.520} &\textbf{0.353} &0.539 & 0.353 & 0.596 &0.368 &0.660  &0.408 &1.181 &0.486\\
\midrule
\multirow{4}{*}{\rotatebox{90}{$Weather$}} 
                        & 96 & 0.199 & 0.262 & \textbf{0.158} & \textbf{0.195} & 0.217  &0.296  &0.266  &0.336 &0.315 &0.288\\
                        & 192 & 0.228 & 0.288 & \textbf{0.211} & \textbf{0.247} & 0.276  &0.336  &0.307  &0.367 &0.341 &0.305\\
                        & 336 &\textbf{0.267} & 0.323 & 0.274 & \textbf{0.300} & 0.339  &0.380  &0.359  &0.395 &0.381 &0.331\\
                        & 720 &\textbf{0.319} & 0.361 &0.351 & \textbf{0.353} & 0.403  &0.428 &0.578 &0.578 &0.440 &0.370 \\
\midrule
\multirow{4}{*}{\rotatebox{90}{$ILI$}} 
                        & 24 & 1.970 & 0.875 & \textbf{1.862} & \textbf{0.869} & 2.203  &0.963  &3.483 &1.287 &6.581 &1.699 \\
                        & 36 & \textbf{1.982} & \textbf{0.859} &2.071 & 0.969 & 2.272  &0.976  &3.103  &1.148 &7.121 &1.882 \\
                        & 48 & \textbf{1.868} & \textbf{0.896} &2.346 & 1.042 & 2.209  &0.981  &2.669  &1.085 &6.567 &1.797 \\
                        & 60 & \textbf{2.057} & \textbf{0.929} &2.560 & 1.073 & 2.545  &1.061  &2.770  &1.125 &5.885 &1.675 \\
\bottomrule
\end{tabular}
\label{tab:multi-benchmarks}
}
% \end{adjustwidth}
%\end{footnotesize}
\end{table*}
\subsection{Ablation univariate forecasting experiments for FEL layers with all six datasets }
As shown in Table \ref{tab:ablation_FEL_full}, although LPU+MLP combining all boosting tricks has slightly better performance than FiLM for the ETTm1 dataset, FiLM remains the most consistent and effective model among all variants across all six datasets. FEL is a much better backbone structure than MLP, LSTM, CNN, and vanilla attention modules. 

%\resizebox{!}{\.5\paperheight}{
\begin{table*}[!h]
\vskip -0.05in
\centering
%\begin{footnotesize}
% \begin{adjustwidth}{-1.5in}{-1in}
\caption{: (Full Benchmark)Ablation studies of FEL layer. The FEL layer is replaced with 4 different variants: MLP, LSTM, CNN, and Transformer.The experiments are performed on ETTm1 and Electricity. The metric of variants is presented in relative value (’+’ indicates degraded performance, ’-’ indicates improved performance).}\vspace{-1mm}
\scalebox{0.8}{
\begin{tabular}{c|c|ccccccccccccccc}
\toprule
\multicolumn{2}{c|}{Methods}&\multicolumn{2}{c|}{FilM}&\multicolumn{2}{c|}{LPU+MLP}&\multicolumn{2}{c|}{LPU+LSTM}&\multicolumn{2}{c|}{LPU+CNN}&\multicolumn{2}{c|}{LPU+attention}\\
\midrule
\multicolumn{2}{c|}{Metric} & MSE  & MAE & MSE & MAE& MSE  & MAE& MSE  & MAE& MSE  & MAE& \\
\midrule

\multirow{4}{*}{\rotatebox{90}{ETTm1}} 

&96  &\textbf{0.029} &\textbf{0.127}  &+0.0\%   & +0.0\%   & +12.1\% & +7.1\%    & +13.5\%   & +9.5\%   & +1.7\%  & +1.6\%  \\
& 192  &\textbf{0.041} &\textbf{0.153}  &-1.5\% & -0.6\%  & +12.2\% & +8.5\%  & +10.8\%   & +7.8\%    & +2.0\%  & +3.3\%  \\
& 336 & \textbf{0.053} & \textbf{0.175} &-1.7\% & -1.7\%  & +4.5\% & +4.0\%    & +10.8\%    & +6.3\%    & +4.5\% & +2.9\%   \\
& 720 &\textbf{0.071}& \textbf{0.205}   &-0.9\%  & -1.0\%  & +5.5\% & +3.4\%  & +8.6\%    & +4.9\%    & +13.8\% & +7.8\%   \\

\midrule
\multirow{4}{*}{\rotatebox{90}{Electricity}} 

&96  &\textbf{0.154}  &\textbf{0.247}  &+155\%  & +81\%   & +160\% & +84\%    & +330\%  & +155\%  & +242\% & +119\%  \\%&--& -- & \\
& 192 &\textbf{0.166} & \textbf{0.258} &+59\% & +39\%   & +121\%  & +67\%   & +224\%  & +117\%  & +264\% & +131\%  \\%&--& --  \\
& 336 & \textbf{0.188}& \textbf{0.283} &+55\%  & +35\%   & +150\%  & +74\%   & +128\%  & +71\% & +183\% & +95\%  \\%&--& -- \\
& 720 & \textbf{0.249}&\textbf{0.341}  &+33\%  & +25\%   & +154\%  & +73\%   & +192\%  & +95\%  & +312\% & +138\%  \\ %&--& --  \\

\midrule
\multirow{4}{*}{\rotatebox{90}{Exchange}} 

&96  &\textbf{0.110}  &\textbf{0.247}  &-13\%  & -12\%   & +51\% & +17\%    & +4.6\%  & -1.2\%  & -4.6\% & -5.8\%  \\%&--& -- & \\
& 192 &\textbf{0.207} & \textbf{0.352} &+7.2\% & +0.0\%   & +69\%  & +32\%   & +29\%  & +12\%  & +22\% & +11\%  \\%&--& --  \\
& 336 & \textbf{0.327}& \textbf{0.461} &+48\%  & +13\%   & +62\%  & +20\%   & +68\%  & +24\% & +72\% & +23\%  \\%&--& -- \\
& 720 & \textbf{0.811}&\textbf{0.708}  &+29\%  & +14\%   & +24\%  & +9.6\%   & +38\%  & +12\%  & +64\% & +27\%  \\ %&--& --  \\

\midrule
\multirow{4}{*}{\rotatebox{90}{Traffic}} 

&96  &\textbf{0.144}  &\textbf{0.215}  &+69\%  & +47\%   & +13\% & +15\%    & +300\%  & +176\%  & +271\% & +161\%  \\%&--& -- & \\
& 192 &\textbf{0.120} & \textbf{0.199} &+17\% & +7.5\%   & +31\%  & +24\%   & +258\%  & +149\%  & +1572\% & +355\%  \\%&--& --  \\
& 336 & \textbf{0.128}& \textbf{0.212} &+6.2\%  & +7.6\%   & +16\%  & +15\%   & +151\%  & +102\% & +1514\% & +368\%  \\%&--& -- \\
& 720 & \textbf{0.153}&\textbf{0.252}  &+38\%  & +28\%   & +11\%  & +7.9\%   & +250\%  & +126\%  & +1048\% & +349\%  \\ %&--& --  \\

\midrule
\multirow{4}{*}{\rotatebox{90}{Weather}} 

&96  &\textbf{0.0012}  &\textbf{0.026}  &+17\%  & +6.2\%   & +16\% & +6.9\%    & +19\%  & +8.1\%  & +21\% & +8.9\%  \\%&--& -- & \\
& 192 &\textbf{0.0014} & \textbf{0.029} &-1.4\% & -2.4\%   & +5.0\%  & +1.7\%   & 0.7\%  & -0.7\%  & +4.3\% & +1.4\%  \\%&--& --  \\
& 336 & \textbf{0.0015}& \textbf{0.030} &+0.0\%  & -0.6\%   & +3.3\%  & +1.3\%   & +2.0\%  & +0.0\% & +3.3\% & +1.3\%  \\%&--& -- \\
& 720 & \textbf{0.0022}&\textbf{0.037}  &+4.6\%  & -0.3\%   & +4.1\%  & -1.6\%   & 3.6\%  & 0.0\%  & +0.0\% & -3.8\%  \\ %&--& --  \\

\midrule
\multirow{4}{*}{\rotatebox{90}{ILI}} 

&96  &\textbf{0.629}  &\textbf{0.538}  &+51\%  & +45\%   & -2.5\% & 9.5\%    & +20\%  & +29\%  & +112\% & +59\%  \\%&--& -- & \\
& 192 &\textbf{0.444} & \textbf{0.481} &+99\% & +58\%   & +25\%  & +24\%   & +84\%  & +56\%  & +360\% & +142\%  \\%&--& --  \\
& 336 & \textbf{0.557}& \textbf{0.584} &+33\%  & +31\%   & +21\%  & +16\%   & +58\%  & +30\% & +702\% & +94\%  \\%&--& -- \\
& 720 & \textbf{0.641}&\textbf{0.644}  &+8.4\%  & +5.4\%   & +23\%  & +18\%   & +42\%  & +22\%  & +74\% & +34\%  \\ %&--& --  \\
\bottomrule
\end{tabular}
\label{tab:ablation_FEL_full}
}
% \end{adjustwidth}
%\end{footnotesize}

\vskip -0.05in
\end{table*}
%}

\subsection{Boosting experiments of LPU with common deep learning backbones for all six datasets}
As shown in Table \ref{tab:boosting}, LPU shows a consistent boosting effect across all selected common deep learning backbones for most datasets. It can be used as a simple and effective build add-on block for long-term time series forecasting tasks. Although without data normalization, pure LPU negatively boosts performance for some cases. 

%\resizebox{!}{\.5\paperheight}{
\vskip -0.1in
% \begin{wraptable}

%\begin{wraptable}[12]{r}{0.7\textwidth}
\begin{table*}[h]
\centering
%\begin{footnotesize}
% \begin{adjustwidth}{-1.5in}{-1in}
\caption{(Full Benchmark) Boosting effect of LPU layer for common deep learning backbones: MLP, LSTM, CNN and Attention.`+` indicates degraded performance.}\vspace{-1mm}
\scalebox{0.80}{
\begin{tabular}{c|c|cccccccccccccccccc}
%\begin{tabular}{c|c|cccccccccc}
\toprule
\multicolumn{2}{c|}{Methods}&\multicolumn{2}{c|}{FEL}&\multicolumn{2}{c|}{MLP}&\multicolumn{2}{c|}{LSTM}&\multicolumn{2}{c|}{lagged-LSTM}&\multicolumn{2}{c|}{CNN}&\multicolumn{2}{c}{Attention}\\
\midrule
% \multicolumn{2}{c|}{Metric} & MSE  & MAE & MSE & MAE& MSE  & MAE& MSE  & MAE& MSE  & MAE& MSE  & MAE&\\
\multicolumn{2}{c|}{Compare} & LPU  & Linear& LPU  & Linear & LPU  & Linear & LPU  & Linear & LPU  & Linear & LPU  & Linear\\
\midrule

\multirow{4}{*}{\rotatebox{90}{ETTm1}} 

&96  &\textbf{0.030}  & +38\%   & 0.034  & +8.0\%  & 0.049 & +73\% & 0.093 & -21\% & 0.116   & -50\%   & 0.243  & -81\% \\
& 192  &\textbf{0.047} & +9.5\% & 0.049  & +30\%  & 0.174 & +32\% & 0.331 & -48\% & 0.101   & +20\%    & 0.387  & -86\% \\
& 336 & 0.063 & +5.8\% & \textbf{0.061}  & +64\%  & 0.119 & +84\% & 0.214 & -19\% & 0.122   & +25\%    & 1.652  & +12\% \\
& 720 &\textbf{0.081} & +1.4\%  & 0.082  & +62\%  & 0.184 & +32\% & 0.303 & -6.5\%  & 0.108   & +13\%    & 4.782  & -61\% \\

\midrule
\multirow{4}{*}{\rotatebox{90}{Electricity}} 

&96  &\textbf{0.213}  & +136\%  & 0.431  & +121\%   & 0.291 & +56\% & 0.739 & -33\% & 0.310  & +43\%  & 0.805 & +23\% \\%&--& --
& 192 &\textbf{0.268} & +32\%   & 0.291 & +239\%   & 0.353  & +17\% & 0.535 & +15\% & 0.380  & +12\%  & 0.938 & +14\% \\%&--& --  \\
& 336 & 0.307& +0.1\%  & \textbf{0.296} & +235\%   & 0.436  & -6.7\% & 0.517 & +23\% & 0.359  & +29\% & 2.043 & -54\% & \\%&--& -- \\
& 720 & \textbf{0.321}& +37\%   & 0.339 & +196\%   & 0.636  & -11\% & 0.492 & +28\% & 0.424  & +18\%  & 9.115 & +298\% \\ %&--& --  \\
               
\midrule
\multirow{4}{*}{\rotatebox{90}{$Exchange$}} 
& 96  & 0.130 & +7.5\% & \textbf{0.110} & -18\% & 0.224 & +6.0\% & 0.521 & -58\% & 0.244 & -18\% & 0.338 & +872\% \\
& 192 & \textbf{0.205} & +39\% & 0.257 & -36\% & 0.787 & -35\% & 1.742 & -66\% & 0.630 & +2.1\% & 0.930 & +278\% \\
& 336 & 0.467 & +9.2\% & \textbf{0.461} & -33\% & 0.964 & +24\% & 2.281 & -38\% & 3.231 & -85\% & 1.067 & +69\%\\
& 720 & \textbf{1.003} & +26\% & 1.981 & -61\% & 2.703 & -29\% & 1.457 & +34\% & 5.531 & +9.7\% & 0.631 & +1831\% \\
\midrule

\multirow{4}{*}{\rotatebox{90}{$Traffic$}} 
&96  &\textbf{0.312} & +18\% & 0.376 & +277\% & 0.215 & +1.2\% & 0.216 & +10\% & 0.543 & -33\% & 0.429 & +210\% \\
& 192 & \textbf{0.141} & +9.6\% & 0.199 & +598\% & 0.177 & +19\% & 0.186 & +17\% & 0.451 & +9.0\% & 0.476 & +176\% \\
& 336 & \textbf{0.143} & +2.5\% & 0.195 & +613\% & 0.192 & +19\% & 0.190 & +11\% & 0.346 & +44\% & 0.377 & +260\% \\
& 720 & \textbf{0.215} & +30\% & 0.240 & +475\% & 0.234 & -1.7\% & 0.250 & +15\% & 0.348 &  +47\% & 0.773 & +171\%\\
\midrule

\multirow{4}{*}{\rotatebox{90}{$Weather$}} 
& 96 & 0.0073 & -38\% & 0.006  & -33\% & 0.006 & -23\% & 0.0070 & -17\% & \textbf{0.0022} & +167\% & 0.0065 &-11\%\\
& 192 & 0.0106 & -64\% & 0.007 & -14\% & 0.0074 & -11\% & \textbf{0.0063} & -19\% & 0.007 & -24\% & 0.0075 & -12\%\\
& 336 & 0.0079 & -37\% & 0.006 & +4.9\% & 0.0056 & +12\% & \textbf{0.0055} & +12\% & 0.0056 & +0.5\% & 0.222 & -69\% \\
& 720 &0.0063 & +0.4\% & 0.006 & +7.6\% & \textbf{0.0062} & +5.3\% & 0.103 & -36\% &0.006 & +4.2\% & 0.037 & -81\% \\
                        
\midrule
\multirow{4}{*}{\rotatebox{90}{$ILI$}} 
& 24 & 1.393 &	+6.1\% & \textbf{1.220} & +36\% & 2.306 & +66\% & 4.189 & -9.2\% & 2.264 & -22\% & 2.249 & +217\% \\
& 36 & 1.242 & -22\% & \textbf{1.185} & +56\% & 2.950 & +44\% & 2.516 & +42\% & 1.841 & -3.0\% & 5.026 & +45\% \\
& 48 & 1.448 & -28\% & \textbf{1.079} & +79\% & 3.385 & +38\% & 3.501 & +16\% & 1.654 & +23\% & 2.838 & +115\% \\
& 60 & 2.089 & -18\% & \textbf{0.986} & +96\%  & 4.031 & +18\% & 4.258 & +10\% & 1.290 & +176\% & 4.978 & +250\% \\
\bottomrule
\end{tabular}
\label{tab:boosting}
}
% \end{adjustwidth}
%\end{footnotesize}
\end{table*}
%\end{wraptable}
%}

\subsection{Ablation univariate forecasting experiments for Low rank approximation with all six datasets}
As shown in Table \ref{tab:FEL_LRA_FULL}, with the low-rank approximation of learnable matrix in the Fourier Enhanced Layer significantly reduces our parameter size, and even improves our model's performance for some datasets.
%\resizebox{!}{\.5\paperheight}{
\begin{table*}[h]

%\begin{wraptable}[9]{r}{0.6\textwidth}
\centering
%\begin{footnotesize}
% \begin{adjustwidth}{-1.5in}{-1in}
\caption{Low-rank Approximation (LRA) univariate forecasting study for frequency enhanced layer: Comp. K=0 means default version without LRA, 1 means the largest compression using K=1.}
%\resizebox{\columnwidth}{!}{
\scalebox{0.75}{
\begin{tabular}{c|c|cccccccccc}
\toprule

\multicolumn{2}{c|}{Comp. K}&\multicolumn{2}{c|}{0}&\multicolumn{2}{c|}{16}&\multicolumn{2}{c|}{4}&\multicolumn{2}{c}{1}\\

\midrule
\multicolumn{2}{c|}{Metric} & MSE  & MAE & MSE & MAE& MSE  & MAE& MSE  & MAE \\
\midrule

% \multirow{4}{*}{\rotatebox{90}{$Exchange$}} 

% &96  &\textbf{0.079} &\textbf{0.204}    &0.083  &0.209  &0.082  &0.208   &0.087    &0.217     \\
% & 192  &\textbf{0.159} &\textbf{0.292}  &0.166  &0.304  &0.166  &0.304   &0.172    &0.309      \\
% & 336 & \textbf{0.270} & \textbf{0.398} &0.340  &0.436  &0.300  &0.413   &0.349    &0.452      \\
% & 720 &\textbf{0.788}& \textbf{0.680}   &1.158  &0.806  &1.147  &0.801   &0.915   &0.719      \\
\multirow{4}{*}{\rotatebox{90}{$ETTm2$}} 

&96&0.065&0.189&0.064&0.185&\textbf{0.064}&\textbf{0.185}&0.064&0.186 \\

&192&0.094&0.233&0.094&0.231&0.093&0.231&\textbf{0.093}&\textbf{0.231} \\

&336&0.124&0.274&0.124&0.270&\textbf{0.124}&\textbf{0.269}&0.124&0.271 \\

&720&0.173&0.323&0.173&0.322&\textbf{0.173}&\textbf{0.322}&0.177&0.328 \\
\midrule

\multirow{4}{*}{\rotatebox{90}{$Electricity$}} 

&96&\textbf{0.154}&\textbf{0.247}&0.211&0.324&0.216&0.331&0.277&0.387 \\

&192&\textbf{0.166}&\textbf{0.258}&0.251&0.352&0.246&0.347&0.334&0.421 \\

&336&\textbf{0.188}&\textbf{0.283}&0.276&0.369&0.302&0.396&0.363&0.440 \\

&720&\textbf{0.249}&\textbf{0.341}&0.336&0.429&0.342&0.436&0.411&0.481 \\

\midrule

\multirow{4}{*}{\rotatebox{90}{$Exchange$}} 

&96&0.110&0.259&0.119&0.273&\textbf{0.104}&\textbf{0.247}&0.105&0.251 \\

&192&0.207&0.352&0.196&0.355&\textbf{0.195}&\textbf{0.349}&0.212&0.372 \\

&336&\textbf{0.327}&\textbf{0.461}&0.388&0.497&0.373&0.491&0.407&0.506 \\

&720&\textbf{0.811}&\textbf{0.708}&0.908&0.767&1.288&0.941&1.840&1.153 \\
\midrule

\multirow{4}{*}{\rotatebox{90}{$Traffic$}} 

&96&\textbf{0.144}&\textbf{0.215}&0.146&0.223&0.154&0.237&0.267&0.373 \\

&192&\textbf{0.120}&\textbf{0.199}&0.121&0.201&0.138&0.231&0.218&0.333 \\

&336&0.128&0.212&\textbf{0.120}&\textbf{0.206}&0.132&0.227&0.216&0.335 \\

&720&\textbf{0.153}&\textbf{0.252}&0.155&0.257&0.154&0.257&0.246&0.366 \\

\midrule

\multirow{4}{*}{\rotatebox{90}{$Weather$}} 

&96&0.0012&0.026&0.0011&0.025&\textbf{0.001}&\textbf{0.025}&0.001&0.025 \\

&192&0.0014&0.029&0.0014&0.028&\textbf{0.001}&\textbf{0.028}&0.001&0.028 \\

&336&0.0015&0.03&0.0015&0.030&\textbf{0.001}&\textbf{0.029}&0.002&0.030 \\

&720&0.0022&0.037&0.0022&0.037&\textbf{0.002}&\textbf{0.037}&0.002&0.037 \\
\midrule

\multirow{4}{*}{\rotatebox{90}{$ILI$}} 

&96&0.629&0.538&\textbf{0.599}&\textbf{0.556}&0.628&0.558&0.630&0.579 \\

&192&\textbf{0.444}&\textbf{0.481}&0.487&0.533&0.508&0.561&0.570&0.612 \\

&336&0.557&0.584&\textbf{0.553}&\textbf{0.565}&0.703&0.696&0.722&0.706 \\

&720&\textbf{0.641}&\textbf{0.644}&0.648&0.641&0.900&0.780&1.493&1.032 \\

\midrule
\multicolumn{2}{c|}{Parameter size}&\multicolumn{2}{c|}{100\%}&\multicolumn{2}{c|}{6.4\%}&\multicolumn{2}{c|}{1.6\%}&\multicolumn{2}{c}{0.4\%}\\
% \multirow{4}{*}{\rotatebox{90}{$Exchange$}}
% &96  &\textbf{0.079}  &\textbf{0.204}  &+15\%  & +6.8\% & +11\% & +5.2\%  & +11\%    & +5.1\% \\
% & 192 &\textbf{0.159} & \textbf{0.292} &-4.6\% & -3.8\% & +7.8\%  & +3.9\%   & +6.8\%    & +3.5\%  \\
% & 336 & \textbf{0.270}& \textbf{0.398}&-4.2\%  & -5.0\% & -3.9\%  & -6.0\%   & -7.2\%    & -8.0\% \\
% & 720 & \textbf{0.830}&\textbf{0.721} &+2.9\%  & +2.8\% & +10\%  &  +6.8\%  & +3.0\%   & +1.7\% \\
\bottomrule
\end{tabular}
\label{tab:FEL_LRA_FULL}
}
%}
% \end{adjustwidth}
%\end{footnotesize}
\end{table*}
%\end{wraptable}
%}

\subsection{Ablation univariate forecasting experiments for frequency mode selection with all six datasets}
Three different mode selection policies are studied for frequency enhanced layer: 1) lowest mode selection: we select $m$ lowest frequency modes to retain. 2) random model selection: we select $m$ frequency modes randomly to retain. 3) lowest with extra high mode selection: we select $0.8\times m$ lowest frequency modes and $0.2\times m$ high-frequency modes randomly to retain. The experimental results are summarized in Table \ref{tab:mode_full} with $m = 64$ for both experiments. The lowest mode selection is the most stable frequency mode selection policy through adding some randomness mode can improve the results for some datasets.

% \begin{wraptable}[16]{r}{0.6\textwidth}
\begin{table*}[h]

% \begin{wraptable}[11]{r}{0.5\textwidth}
\vskip -0.1in

\centering
\caption{Mode selection policy study for frequency enhanced layer. Lowest: select the lowest $m$ frequency mode; Random: select $m$ random frequency mode; Low random: select the $0.8*m$ lowest frequency mode and $0.2*m$ random high frequency mode.}\vspace{-1.5mm}
\scalebox{0.75}{
\begin{tabular}{c|c|cccccccc}
\toprule
\multicolumn{2}{c|}{Policy}&\multicolumn{2}{c|}{Lowest}&\multicolumn{2}{c|}{Random}&\multicolumn{2}{c}{Low random}\\
\midrule
\multicolumn{2}{c|}{Metric} & MSE  & MAE & MSE & MAE& MSE  & MAE \\
\midrule
\multirow{4}{*}{\rotatebox{90}{ETTm2}} 
&96&\textbf{0.065}&\textbf{0.189}&0.066&0.189&0.066&0.190 \\

&192&\textbf{0.094}&\textbf{0.233}&0.096&0.235&0.096&0.235 \\

&336&\textbf{0.124}&0.274&0.125&\textbf{0.270}&0.128&0.275 \\

&720&0.173&0.323&\textbf{0.173}&\textbf{0.322}&0.173&0.323 \\

\midrule
\multirow{4}{*}{\rotatebox{90}{Electricity}} 
&96&\textbf{0.154}&\textbf{0.247}&0.175&0.0.260&0.176&0.262 \\

&192&\textbf{0.166}&\textbf{0.258}&0.177&0.266&0.168&0.273 \\

&336&\textbf{0.188}&\textbf{0.283}&0.199&0.289&0.192&0.299 \\

&720&\textbf{0.249}&\textbf{0.341}&0.269&0.364&0.270&0.362 \\

\midrule
\multirow{4}{*}{\rotatebox{90}{Exchange}} 
&96&0.11&0.259&0.110&0.256&\textbf{0.106}&\textbf{0.249} \\

&192&0.207&0.352&\textbf{0.196}&\textbf{0.351}&0.207&0.357 \\

&336&\textbf{0.327}&\textbf{0.461}&0.451&0.522&0.373&0.484 \\

&720&0.811&0.708&0.835&0.714&\textbf{0.604}&\textbf{0.628} \\

\midrule
\multirow{4}{*}{\rotatebox{90}{Traffic}} 
&96&\textbf{0.144}&\textbf{0.215}&0.145&0.216&0.145&0.217 \\

&192&0.12&0.199&0.119&0.198&\textbf{0.118}&\textbf{0.197} \\

&336&0.128&0.212&\textbf{0.122}&\textbf{0.207}&0.122&0.209 \\

&720&0.153&0.252&\textbf{0.142}&\textbf{0.238}&0.155&0.259 \\

\midrule
\multirow{4}{*}{\rotatebox{90}{Weather}} 
&96&\textbf{0.0012}&\textbf{0.026}&0.0012&0.027&0.0012&0.026 \\

&192&\textbf{0.0014}&\textbf{0.029}&0.0014&0.029&0.0014&0.029 \\

&336&\textbf{0.0015}&\textbf{0.03}&0.0015&0.030&0.0015&0.030 \\

&720&\textbf{0.0022}&\textbf{0.037}&0.0023&0.037&0.0023&0.037 \\

\midrule
\multirow{4}{*}{\rotatebox{90}{ILI}} 
&96&0.629&0.538&0.639&0.542&\textbf{0.626}&\textbf{0.537} \\

&192&\textbf{0.444}&\textbf{0.481}&0.448&0.490&0.447&0.494 \\

&336&\textbf{0.557}&\textbf{0.584}&0.560&0.590&0.557&0.587 \\

&720&\textbf{0.641}&\textbf{0.644}&0.641&0.647&0.643&0.650 \\

\bottomrule

\end{tabular}
\label{tab:mode_full}
}
\end{table*}
% \end{wraptable}
