# Supplementary material for: Sparse-VQ Transformer: An FFN-Free Framework with Vector Quantization for Enhanced Time Series Forecasting
Source: arXiv:2402.05830 source file (2024-02-08)
Supplement: Supplementary file 5 [file algorithms.tex]

\section{Algorithm Implementation}
\label{app:Alg}
\input{figures/algorithm_0}
%\paragraph{Implementation for Frequency Enhanced Layer}
\input{figures/algorithm_1}
