# Supplementary material for: Sparse-VQ Transformer: An FFN-Free Framework with Vector Quantization for Enhanced Time Series Forecasting
Source: arXiv:2402.05830 source file (2024-02-08)
Supplement: Supplementary file 9 [file noise_injection.tex]

\section{Noise Injection Experiment}
\label{app:noise}
Our model's robustness in long-term forecasting tasks can be demonstrated using a series of noise injection experiments as shown in Table \ref{tab:ablation_noise}. As we can see, adding Gaussian noise in the training/test stage has a limited effect on our model's performance, since the %average 
deterioration is less than 1.5\% in the worst case. The model's robustness is consistent across various forecasting horizons. Note that adding the noise in the testing stage other than the training stage will even improve our performance by 0.4\%, which further supports our claim of robustness. 
%\resizebox{!}{\.5\paperheight}{
\begin{table*}[h]
\centering
%\begin{footnotesize}
% \begin{adjustwidth}{-1.5in}{-1in}
\caption{Noise injection studies. A 0.3*$\mathcal{N}\left(0,1\right)$ Gaussian noise is introduced into our training/testing. We conduct 4 sets of experiments with/without noise in training and test phases. The experiments are performed on ETTm1 and Electricity with different output lengths. The metric of variants is presented in relative value ('+' indicates degraded performance, and '-' indicates improved performance).}
%\resizebox{\columnwidth}{!}{
\scalebox{0.75}{
\begin{tabular}{c|c|cccccccc}
\toprule

\multicolumn{2}{c|}{Training}&\multicolumn{4}{c|}{noise}&\multicolumn{4}{c}{with noise}\\
\midrule
\multicolumn{2}{c|}{Testing}&\multicolumn{2}{c|}{without noise}&\multicolumn{2}{c|}{with noise}&\multicolumn{2}{c|}{without noise}&\multicolumn{2}{c}{with noise}\\

\midrule
\multicolumn{2}{c|}{Metric} & MSE  & MAE & MSE & MAE& MSE  & MAE& MSE  & MAE \\
\midrule
% \multirow{4}{*}{\rotatebox{90}{$ETTm2$}} &96 & \textbf{0.165} & \textbf{0.256} &0.203 &0.287 &0.255  &0.339 &0.705 &0.690 &0.365  &0.453  &0.768  &0.642  &0.658  &0.619    \\
%                         & 192 & \textbf{0.240} & \textbf{0.313} &0.269  &0.328  &0.281 &0.340 &0.924 &0.692 &0.533  &0.563  &0.989  &0.757  &1.078  &0.827    \\
%                         & 336 & \textbf{0.286} & \textbf{0.345} & 0.325 &0.366 &0.339  &0.372 &1.364 &0.877 &1.363&0.887  &1.334  &0.872  &1.549  &0.972     \\
%                         & 720 & \textbf{0.393} & \textbf{0.410} &0.421 &0.415 &0.422  &0.419 &0.877 &1.074 &3.379  &1.338 & 3.048 &1.328  &2.631  &1.242      \\
% \midrule
\multirow{4}{*}{\rotatebox{90}{$ETTh1$}} 

&96  &\textbf{0.371} &\textbf{0.394}    &-1.6\%  & -2.0\% & -0.0\% & -0.0\%  & -1.6\%   & -2.0\%     \\
& 192  &\textbf{0.414} &\textbf{0.423}  &-0.5\%  & -1.4\%    & +0.5\% & -0.0\%  & -0.5\%   & -1.4\%    \\
& 336 & \textbf{0.442} & \textbf{0.445} &-1.8\% & -0.9\%    & -0.9\% & +1.3\%  & -3.2\%   & -1.6\%     \\
& 720 &\textbf{0.465}& \textbf{0.472}   &+0.2\%     & -0.2\%     &+0.9\%    & +0.9\%  & -0.6\%    & -0.4\%    \\

% \midrule

% \multirow{4}{*}{\rotatebox{90}{$Exchange$}}
% &96  &\textbf{0.079}  &\textbf{0.204}  &+15\%  & +6.8\% & +11\% & +5.2\%  & +11\%    & +5.1\% \\
% & 192 &\textbf{0.159} & \textbf{0.292} &-4.6\% & -3.8\% & +7.8\%  & +3.9\%   & +6.8\%    & +3.5\%  \\
% & 336 & \textbf{0.270}& \textbf{0.398}&-4.2\%  & -5.0\% & -3.9\%  & -6.0\%   & -7.2\%    & -8.0\% \\
% & 720 & \textbf{0.830}&\textbf{0.721} &+2.9\%  & +2.8\% & +10\%  &  +6.8\%  & +3.0\%   & +1.7\% \\
\bottomrule
\end{tabular}
\label{tab:ablation_noise}
}
%}
% \end{adjustwidth}
%\end{footnotesize}
\end{table*}
%}
