# Supplementary material for: Sparse-VQ Transformer: An FFN-Free Framework with Vector Quantization for Enhanced Time Series Forecasting
Source: arXiv:2402.05830 source file (2024-02-08)
Supplement: Supplementary file 10 [file parameter_sensitivity.tex]

\section{Parameter Sensitivity}
\label{app:parameter}
\paragraph{Influence of Legendre Polynomial number $N$ and Frequency mode number $M$}
\begin{figure*}[h]
    \centering
    \includegraphics[width=0.8\linewidth]{figures/MSE_vs_N/N_vs_dataset_all_15.eps}
    \caption{The reconstruction error (MSE) vs. Legendre Polynomial number ($N$) on three datasets with three different input lengths.}
    \label{fig:MSE_vs_Hippo_N}
\end{figure*}
The experimental results on three different datasets (ETTm1, Electricity, and Exchange) in Figure \ref{fig:MSE_vs_Hippo_N} show the optimal choice of Legendre Polynomials number ($N$) when we aim to minimize the reconstruction error (in MSE) on the historical data. The MSE error decreases sharply at first and saturates at an optimal point, where $N$ is in proportion to the input length. For input sequences with lengths of 192, 336, and 720, $N$ $\approx$ 40, 60, and 100 gives the minimal MSE,  respectively. %We select a default N = 256 to give our model enough representation powder for a long term historical signal recover with multiscale mechanism implemented.

\begin{figure*}[h]
    \centering
    % \includegraphics{figures/MSE_vs_N/elc_192.eps}
    % (a)
    \includegraphics[width=0.99\linewidth]{figures/N_vs_modes/N_vs_modes_all_ecl.eps}
    % (b)
    % \includegraphics[width=0.28\linewidth]{figures/N_vs_modes/N_vs_modes_pr336_ecl.eps}
    % (c)
    % \includegraphics[width=0.28\linewidth]{figures/N_vs_modes/N_vs_modes_pr720_ecl.eps}
    \caption{The MSE error of univariate time series forecasting task on Electricity dataset with different Legendre Polynomials number ($N$), mode number and input length. Left: input length = 192. Mid: input length = 336. Right: input length = 720.}
    \label{fig:MSE_vs_modes_vs_N}
\end{figure*}

Figure \ref{fig:MSE_vs_modes_vs_N} shows the MSE error of time series forecasting on the Electricity dataset, with different Legendre Polynomials number ($N$), mode number, and input length. We observe that, when enlarging $N$, the model performance saturates at an optimal point. For example, in Figure \ref{fig:MSE_vs_modes_vs_N} Left (input length=192), the best performance is reached when $N>64$. While in Figure \ref{fig:MSE_vs_modes_vs_N} Right (input length=720), the best performance is reached when $N$ is larger than 128. Another influential parameter is the mode number. From Figure \ref{fig:MSE_vs_modes_vs_N} we observe that a small mode number will lead to better performance, as a module with a small mode number works as a denoising filter.
