# Supplementary material for: Sparse-VQ Transformer: An FFN-Free Framework with Vector Quantization for Enhanced Time Series Forecasting
Source: arXiv:2402.05830 source file (2024-02-08)
Supplement: Supplementary file 11 [file proof_fourier.tex]

% \section{Proof of Theorem \ref{thm_Fourier}}

% \begin{theorem*}
% \label{thm_Fourier_correct} 
% Let $A\in\mathbbm{R}^{d\times n}$ be the Fourier coefficients matrix of an input matrix $X\in\mathbbm{R}^{d\times n}$, and $\mu(A)$, the coherence measure of matrix $A$, is $\Omega(k/n)$. We assume there exist $s$ and  a positive $ a_{\min}$ such that the elements in last $n-s$ columns of $A$ is smaller than $a_{\min}$. If we keep first $s$ columns selected and randomly choose $\mathcal{O}(k^2/\epsilon^2 - s)$ columns from the remaining parts, with high probability
% \[
%     \|A - P(A)\|_F \leq \mathcal{O}\left[(1 + \epsilon)a_{\min}\cdot\sqrt{(n-s)d}\right],
% \]
% where  $P(A)$ denotes the matrix projecting $A$ onto the column selected column space.
% \end{theorem*}
% (In Theorem \ref{thm_Fourier_correct}, we correct a typo error in Theorem \ref{thm_Fourier}. The ``in last d - s columns...'' should be ``in last n - s columns...''). 

% \begin{proof}
% Similar to the analysis in Appendix C of~\cite{FedFormer}, let $A_k = P(A)$ and $A_{\bar{k}}$ be the matrix projecting A onto the remaining-column space, where the columns are not selected. $A = A_k + A_{\bar{k}}$. So we have $\|A - P(A)\|_F = \| A_{\bar{k}}\|$. In the assumption of Theorem \ref{thm_Fourier_correct}, the elements in $A_{\bar{k}}$ is smaller than $a_{\min}$, thus $\| A_{\bar{k}}\|_F = \sqrt{\mathrm{trace}(A_{\bar{k}}^\top \cdot A_{\bar{k}})} \leq a_{\min} \cdot \sqrt{(n-s)d}$. ($A_{\bar{k}} \in \mathbb{R}^{d \times (n-s)}$)
% \end{proof}
% % In we observe that 

\section{Theoretical Analysis}

\subsection{Theorem 1}
The proof is a simple extension of Proposition 6 in \cite{Hippo}. We omit it for brevity.

\subsection{Theorem 2}
% In order to generate a stable sequence $\{x_t\}$, we restrict the matrix $A$ to be unitary. The above Theorem indicates that the uncertain portion between $x_{t}$  and its estimation $A^{\theta}x_{t-\theta} + \sum_{i=1}^{\theta-1}A^{i}b$ at time $t-\theta$ is scaled with $\sqrt{\theta}$. The larger $\theta$ will lead to higher uncertainty and it in turn leads less correlation between $x_t$ and $x_{t-\theta}$. Therefore introducing more historical information may not necessary lead better performance.
As we have $x_t = Ax_{t-1} + b - \epsilon_{t-1}$ for $t=2,3,...\theta$, we recursively use them and the following result holds:
\begin{align}
    x_{t} &= Ax_{t-1} +  b + \epsilon_{t-1}\notag\\
    &= A(Ax_{t-2} +  b + \epsilon_{t-2})+  b + \epsilon_{t-1}\notag\\
    &=A^2x_{t-2} + Ab + b + A\epsilon_{t-2} + \epsilon_{t-1}\notag\\
    % &=A^3x_{t-3} +  A^2b  + Ab + b + A^2\epsilon_{t-3}+ A\epsilon_{t-2} + \epsilon_{t-1}\notag\\
    &\cdots\notag\\
    &=A^{\theta}x_{t-\theta} + \sum_{i=1}^{\theta-1}A^ib+ \underbrace{\sum_{i=1}^{\theta-1}A^i\epsilon_{t-i}}_{(*)}\notag.
\end{align}
Following Hoeffding inequality, for $\mu>0$ we have
\begin{align}
    \mathbbm{P}\left(|(*)|\ge \mu\right)\le \exp\left(-\frac{2\mu^2}{\sum_{i=1}^{\theta -1}\|A^i\epsilon_{t-1}\|_{\psi_2}^2}\right),
\end{align}
where $\|\cdot\|_{\psi_2}$ is the Orlicz norm defined as
\begin{align}
    \|X\|_{\psi_2} :=\inf\left\{c\ge 0: \mathbbm{E}[\exp(X^2/c^2)]\le 2\right\}\notag.
\end{align}
Since we require $A$ being unitary, we will have $\|A\epsilon\|_2^2 = \|\epsilon\|_2^2$ and it implies $\|A^i\epsilon_{t-1}\|_{\psi_2}^2\| = \|\epsilon_{t-1}\|_{\psi_2}^2 =   \mathcal{O}(\sigma^2)$ for $i=1,2,...,\theta$. The desirable result follows by setting $\mu = \mathcal{O}(\sqrt{\theta}\sigma)$.

\subsection{Theorem 3}

% \begin{theorem*}
% \label{thm_Fourier_correct} 
% Let $A\in\mathbbm{R}^{d\times n}$ be the Fourier coefficients matrix of an input matrix $X\in\mathbbm{R}^{d\times n}$, and $\mu(A)$, the coherence measure of matrix $A$, is $\Omega(k/n)$. We assume there exist $s$ and  a positive $ a_{\min}$ such that the elements in last $n-s$ columns of $A$ is smaller than $a_{\min}$. If we keep first $s$ columns selected and randomly choose $\mathcal{O}(k^2/\epsilon^2 - s)$ columns from the remaining parts, with high probability
% \[
%     \|A - P(A)\|_F \leq \mathcal{O}\left[(1 + \epsilon)a_{\min}\cdot\sqrt{(n-s)d}\right],
% \]
% where $P(A)$ denotes the matrix projecting $A$ onto the column selected column space.
% \end{theorem*}
% (In Theorem \ref{thm_Fourier_correct}, we correct a typo error in Theorem \ref{thm_Fourier}. The ``in last d - s columns...'' should be ``in last n - s columns...''). 

% \begin{proof}
As we keep first $s$ columns selected, $P(A)-A$ has all $0$ elements in first $s$ columns. We thus ignore them and consider the approximation quality on $\tilde{A}\in\mathbb{R}^{d\times (n-s)}$ with the sampled columns.  Via the similar analysis in Appendix C of \cite{FedFormer}, with high probability we have $\| \tilde{A}-P(A) \|_F \leq (1+\epsilon) \|\tilde{A} - \tilde{A}_k\|_F$, where $\tilde{A}_k$ is the ``best” rank-$k$ approximation provided by truncating the singular value decomposition (SVD) of $\tilde{A}$, and where $\|\cdot\|_F$
is the Frobenius norm. As we assume the element in last $n - s$ columns of $A$ is smaller than $a_{\min}$, one can verify  $\| \tilde{A}-P(A) \|_F\le \sqrt{d \times (n-s)}a_{\min}$ and desirable result follows immediately.  
% \end{proof}
